# Supplementary material for: Proximity Sensing: Modeling and Understanding Noisy RSSI-BLE Signals and Other Mobile Sensor Data for Digital Contact Tracing
Source: arXiv:2009.04991 source file (2020-12-24)
Supplement: Supplementary file 1 [file appendix.tex]

\section{Appendix}
\label{appendix}

  %The code for the experiments performed in this paper is available here: <github>

% TODO - REWORD WHATEVER IS PASTED BELOW AS IT IS A DIRECT COPY PASTE

%we also notice that the ConvGRU has excellent results onthe NIST dataset, but siginificantly lost performance on theMITRE dataset.nals due to missing devices.

\begin{table}[!hbt]
\begin{tabular}{|c|c|c|c|c|c|}
\hline
\textbf{Method}     & \textbf{Num Layers} & \textbf{Epochs} & \textbf{\begin{tabular}[c]{@{}c@{}}Hidden\\  Size\end{tabular}} & \textbf{Learning Rate} & \textbf{\begin{tabular}[c]{@{}c@{}}Batch\\  Size\end{tabular}} \\ \hline
ConvGRU             & 2                   & 200             & 200                                                             & 1.00E-03               & 25                                                             \\ \hline
ConvGRU             & 2                   & 200             & 10                                                              & 1.00E-03               & 25                                                             \\ \hline
ConvGRU             & 1                   & 200             & 5                                                               & 1.00E-03               & 25                                                             \\ \hline
ConvGRU             & 2                   & 200             & 200                                                             & 1.00E-03               & 200                                                            \\ \hline
ConvGRU             & 2                   & 200             & 200                                                             & 1.00E-04               & 1000                                                           \\ \hline
ConvGRU             & 2                   & 200             & 200                                                             & 1.00E-04               & 1000                                                           \\ \hline
ConvGRU (no linear) & 2                   & 500             & 200                                                             & 1.00E-04               & 4000                                                           \\ \hline
ConvGRU (no linear) & 2                   & 200             & 200                                                             & 1.00E-04               & 500                                                            \\ \hline
ConvGRU (no linear) & 2                   & 500             & 200                                                             & 1.00E-04               & 4000                                                           \\ \hline
Plain GRU           & 2                   & 40              & 200                                                             & 3.00E-04               & 100                                                            \\ \hline
Plain LSTM          & 2                   & 40              & 200                                                             & 3.00E-04               & 100                                                            \\ \hline
Conv 1d             & 1 conv + 2 linear   & 100             & 64                                                              & 1.00E-05               & 50                                                             \\ \hline
Conv 1d             & 1 conv + 2 linear   & 100             & 64                                                              & 1.00E-04               & 50                                                             \\ \hline
Conv 1d             & 1 conv + 2 linear   & 148             & 64                                                              & 1.00E-05               & 50                                                             \\ \hline
Conv1D (Dilated)    & 3 conv + 2 linear   & 100             & 64                                                              & 1.00E-05               & 50                                                             \\ \hline
Conv1D (Dilated)    & 3 conv + 2 linear   & 100             & 64                                                              & 1.00E-05               & 128                                                            \\ \hline
Conv1D (MaxPool)    & 3 conv + 2 linear   & 100             & 64                                                              & 1.00E-05               & 128                                                            \\ \hline
\caption{The hyper-parameter tuning setup experimented across the models.}
\end{tabular}
\end{table}
% The best results for the RNN style models are obtained using 2 layers and a hidden size of 200 (learning rate =  3.00E-04), and a kernel size of 3 for the ConvGRU. The best results for the feed forward network are obtained by using 2 layers and a learning rate of 1.00E-04.
